# Supplementary material for: Parity-dependent unidirectional and chiral photon transfer in reversed-dissipation cavity optomechanics
Source: arXiv:2212.12085 ancillary file (2022-12-22)
Supplement: Supplementary file 1 [file Supplementary_materials.pdf]

# Supplementary Materials for
# Parity-dependent unidirectional and chiral photon transfer in reversed-dissipation cavity optomechanics


Zhen Chen[a], Qichun Liu[a], Jingwei Zhou[b], Peng Zhao[a], Haifeng Yu[a,*], Tiefu Li[c,a,*], Yulong Liu[a,*]

[a]Beijing Academy of Quantum Information Sciences, Beijing, 100193, China
[b]CAS Key Laboratory of Microscale Magnetic Resonance, University of Science and Technology of China, Hefei, 230026, China
[c]School of Integrated Circuits and Frontier Science Center for Quantum Information, Tsinghua University, Beijing, 100084, China


## 1. An effective Hamiltonian for multimode cavity optomechanics in the reversed-dissipation regime

As discussed in the main text, the original Hamiltonian for the multimode cavity optomechanical system can be expressed as

$$
\begin{aligned}
H &= \omega_a a^\dagger a + \omega_b b^\dagger b + \omega_m m^\dagger m + G(a^\dagger b + b^\dagger a) \\
&\quad -g_a a^\dagger a(m^\dagger + m) - g_b b^\dagger b(m^\dagger + m) \\
&\quad +i\varepsilon_1(a^\dagger e^{-i\Omega_a t} - a e^{i\Omega_a t}) \\
&\quad +i\varepsilon_2(b^\dagger e^{-i\Omega_b t} - b e^{i\Omega_b t})
\end{aligned} \tag{S1}
$$

where $g_a$ ($g_b$) is the single-photon optomechanical strength between the mode $a$ ($b$) and the mechanical mode $m$. The last two terms in Eq. (S1) describe the coupling between two pump laser fields with frequency $\Omega_{a,b}$ and the cavity fields, where $\varepsilon_1$ ($\varepsilon_2$) is the amplitude of the driving field. In the rotating frame at the frequency $\Omega_r = (\Omega_a + \Omega_b)/2$, the Hamiltonian becomes

$$
\begin{aligned}
H &= \Delta_a a^\dagger a + \Delta_b m^\dagger m + \omega_m b^\dagger b + G(a^\dagger b + b^\dagger a) \\
&\quad -g_a a^\dagger a(m^\dagger + m) - g_a b^\dagger b(m^\dagger + m) \\
&\quad +i(\varepsilon_1 a^\dagger e^{-i\delta_r t} - \varepsilon_1^* a e^{i\delta_r t}) \\
&\quad +i(\varepsilon_2 b^\dagger e^{i\delta_r t} - \varepsilon_2^* b e^{-i\delta_r t}),
\end{aligned} \tag{S2}
$$

Here, $\Delta_a(\Delta_b) = \omega_a(\omega_b) - \Omega_r$ is the detuning between the mode $a$ ($b$) and the driving field at frequency $\Omega_r$. $\delta_r = (\Omega_a - \Omega_b)/2$ represents the frequency detuning between these two pump tones. In the following discussions, the cavity modes are assumed to be degenerate, viz., $\omega_a = \omega_b$. Then the detuning parameters become $\Delta_a = \Delta_b = \Delta$, and $\delta_r$ is zero.

The dynamics of the system are determined by the following Langevin equations

$$\dot{a} = -(\kappa_1 + i\Delta)\, a - iGb + ig_a(m^\dagger + m)a + \varepsilon_1, \tag{S3}$$

$$\dot{b} = -(\kappa_2 + i\Delta)\, b - iGa + ig_b(m^\dagger + m)b + \varepsilon_2, \tag{S4}$$

$$\dot{m} = -(\gamma + i\omega_m)\, m + ig_a a^\dagger a + ig_b b^\dagger b, \tag{S5}$$

Here, the input quantum noises have been neglected. The steady-state solutions to Eqs. (S3)-(S5) can be obtained by setting the time derivatives to zero. In addition, these equations can be linearized by writing each operator the sum of


*Corresponding author
*Email addresses:* hfyu@baqis.ac.cn (Haifeng Yu), litf@tsinghua.edu.cn (Tiefu Li), liuyl@baqis.ac.cn (Yulong Liu)

its steady-state solution and a small fluctuation, i.e., $a = \alpha + \delta a$, $b = \beta + \delta b$, and $m = \mu + \delta m$. Subsequently, we have

$$\begin{aligned}
\delta\dot{a} &= -\left(\kappa_1 + i\bar{\Delta}_a\right)\delta a - iG\delta b + iG_a(\delta m^\dagger + \delta m), \quad &(S6)\\
\delta\dot{b} &= -\left(\kappa_2 + i\bar{\Delta}_b\right)\delta b - iG\delta a + iG_b(\delta m^\dagger + \delta m), \quad &(S7)\\
\delta\dot{m} &= -(\gamma + i\omega_m)\delta m + i(G_a^*\delta a + G_a\delta a^\dagger)\\
&\quad + i(G_b^*\delta b + G_b\delta b^\dagger), \quad &(S8)
\end{aligned}$$

where $\bar{\Delta}_a = \Delta - g_a(\mu^* + \mu)$, $\bar{\Delta}_b = \Delta - g_b(\mu^* + \mu)$ are the effective detunings including the radiation pressure effect. $G_a = g_a\alpha$, $G_b = g_b\beta$ are the linearized optomechanical couplings strengths. Moving Eqs. (S6)-(S8) into another interaction picture, i.e., by introducing the slowly moving operators with tildes, viz., $\delta a = \delta\tilde{a}e^{-i\bar{\Delta}_a t}$, $\delta b = \delta\tilde{b}e^{-i\bar{\Delta}_b t}$, and $\delta m = \delta\tilde{m}e^{-i\omega_m t}$, we obtain the following quantum Langevin equations:

$$\begin{aligned}
\delta\dot{\tilde{a}} &= -\kappa_1\delta\tilde{a} - iG\delta\tilde{b}\\
&\quad + iG_a\left[\delta\tilde{m}^\dagger e^{i(\bar{\Delta}_a+\omega_m)t} + \delta\tilde{m}e^{i(\bar{\Delta}_a-\omega_m)t}\right], \quad &(S9)\\
\delta\dot{\tilde{b}} &= -\kappa_2\delta\tilde{b} - iG\delta\tilde{a}\\
&\quad + iG_b\left[\delta\tilde{m}^\dagger e^{i(\bar{\Delta}_b+\omega_m)t} + \delta\tilde{m}e^{i(\bar{\Delta}_b-\omega_m)t}\right], \quad &(S10)\\
\delta\dot{\tilde{m}} &= -\gamma\delta\tilde{m}\\
&\quad + i\left[G_a^*\delta\tilde{a}e^{-i(\bar{\Delta}_a-\omega_m)t} + G_a\delta\tilde{a}^\dagger e^{i(\bar{\Delta}_a+\omega_m)t}\right]\\
&\quad + i\left[G_b^*\delta\tilde{b}e^{-i(\bar{\Delta}_b-\omega_m)t} + G_b\delta\tilde{b}^\dagger e^{i(\bar{\Delta}_b+\omega_m)t}\right], \quad &(S11)
\end{aligned}$$

Because $\bar{\Delta}_a(\bar{\Delta}_b) + \omega_m > G_a, G_b, \kappa_1, \kappa_2, \gamma$, we can invoke the rotating wave approximation (RWA),

$$\begin{aligned}
\delta\dot{\tilde{a}} &= -\kappa_1\delta\tilde{a} - iG\delta\tilde{b} + iG_a\delta\tilde{m}e^{i(\bar{\Delta}_a-\omega_m)t}, \quad &(S12)\\
\delta\dot{\tilde{b}} &= -\kappa_2\delta\tilde{b} - iG\delta\tilde{a} + iG_b\delta\tilde{m}e^{i(\bar{\Delta}_b-\omega_m)t}, \quad &(S13)\\
\delta\dot{\tilde{m}} &= -\gamma\delta\tilde{m} + iG_a^*\delta\tilde{a}e^{-i(\bar{\Delta}_a-\omega_m)t}\\
&\quad + iG_b^*\delta\tilde{b}e^{-i(\bar{\Delta}_b-\omega_m)t}, \quad &(S14)
\end{aligned}$$

In our system, the mechanical mode $m$ is in the *reversed-dissipation regime* and almost decoupled from the system. Thus, Eqs. (S12)-(S14) can be adiabatically eliminated as follows.

According to Eq. (S14), we can obtain the formal solution of $\delta\tilde{b}(t)$ as

$$\begin{aligned}
\delta\tilde{m}(t) = e^{-\gamma t}\int_0^t &\left[iG_a^*\delta\tilde{a}(\tau)e^{-i(\bar{\Delta}_a-\omega_m)\tau+\gamma\tau}\right.\\
&\left. + iG_b^*\delta\tilde{b}(\tau)e^{-i(\bar{\Delta}_b-\omega_m)\tau+\gamma\tau}\right]d\tau. \quad (S15)
\end{aligned}$$

The reversed-dissipation mode $m$ leads to the condition $\gamma > \kappa_1, \kappa_2$. Therefore, $\delta\tilde{m}(t)$ evolves much faster than $\delta\tilde{a}(t)$ and $\delta\tilde{b}(t)$. Then we can set $\delta\tilde{a}(\tau) \approx \delta\tilde{a}(t)$, $\delta\tilde{b}(\tau) \approx \delta\tilde{b}(t)$, and take them out of the integral in Eq. (S15) to obtain

$$\begin{aligned}
\delta\tilde{m}(t) &= \frac{iG_a^*\delta\tilde{a}(t)}{\gamma - i(\bar{\Delta}_a - \omega_m)}e^{-i(\bar{\Delta}_a-\omega_m)t}\\
&\quad + \frac{iG_b^*\delta\tilde{b}(t)}{\gamma - i(\bar{\Delta}_b - \omega_m)}e^{-i(\bar{\Delta}_b-\omega_m)t}. \quad (S16)
\end{aligned}$$

Substituting Eq. (S16) into Eqs. (S12)-(S13), we can adiabatically eliminate the mechanical mode $m$ to obtain the following equations of motion for the cavity modes $\delta\tilde{a}$ and $\delta\tilde{b}$:

$$\begin{aligned}
\delta\dot{\tilde{a}} &= -\left(\kappa + \frac{|G_a|^2}{\gamma}\right)\delta\tilde{a} - \left(\frac{G_aG_b^*}{\gamma} + iG\right)\delta\tilde{b}, \quad &(S17)\\
\delta\dot{\tilde{b}} &= -\left(\frac{G_a^*G_b}{\gamma} + iG\right)\delta\tilde{a} - \left(\kappa + \frac{|G_b|^2}{\gamma}\right)\delta\tilde{b}, \quad &(S18)
\end{aligned}$$

where we have set $\bar{\Delta}_a = \bar{\Delta}_b = \omega_m = \Delta, \kappa_1 = \kappa_2 = \kappa$. Transforming back to the original picture with $\delta\tilde{a} = \delta a e^{i\Delta t}$ and $\delta\tilde{b} = \delta b e^{i\Delta t}$, we can obtain

$$\delta\dot{a} = -\left(\kappa + i\Delta + \frac{|G_a|^2}{\gamma}\right)\delta a - (\frac{G_a G_b^*}{\gamma} + iG)\delta b, \tag{S19}$$

$$\delta\dot{b} = -(\frac{G_a^* G_b}{\gamma} + iG)\delta a - \left(\kappa + i\Delta + \frac{|G_b|^2}{\gamma}\right)\delta b \tag{S20}$$

There, the effective Hamiltonian for the two cavity modes can be given by

$$\begin{aligned} H_{\text{eff}} &= \left[\Delta - i(\kappa + \frac{|G_a|^2)}{\gamma}\right] a^\dagger a + \left[\Delta - i(\kappa + \frac{|G_b|^2}{\gamma})\right] b^\dagger b \\ &\quad + G(a^\dagger b + b^\dagger a) + i\frac{G_a G_b^*}{\gamma} a^\dagger b + i\frac{G_a^* G_b}{\gamma} a b^\dagger \\ &= [(\Delta - i(\kappa + J)] a^\dagger a + [(\Delta - i(\kappa + J)] b^\dagger b \\ &\quad + G(a^\dagger b + b^\dagger a) + iJ(a^\dagger b e^{-i\theta} + a b^\dagger e^{i\theta}). \end{aligned} \tag{S21}$$

Here, we assume $|G_a| = |G_b|$ and $J = |G_a|^2/\gamma$. Note that both $G_a$ and $G_b$ are complex numbers whose phases depend on $\varepsilon_1$ and $\varepsilon_2$. Therefore, the phase $\theta = \arg(G_a^* G_b/\gamma)$ can be well controlled by the two driving tones. In addition to using optomechanical interactions, such a conjugate Peierls phase for exchange couplings can also be realized through nonlinear parametric processes, e.g., four-wave-mixing [1, 2].

## 2. Destructive interference between the coherent and dissipative couplings

The interaction Hamiltonian of coupled resonant modes $a$ and $b$ can be treated as

$$H_{\text{I}} = H_{\text{s}} + H_{\text{a}}, \tag{S22}$$

where the interaction Hamiltonian to describe the coherent coupling is

$$H_{\text{s}} = G(\text{a}^\dagger b + G b^\dagger a), \tag{S23}$$

and the reversed-dissipation mechanical mode mediated dissipative interaction Hamiltonian is given by

$$H_{\text{a}} = iJ\left(\text{e}^{-i\theta} a^\dagger b + e^{i\theta} b^\dagger a\right). \tag{S24}$$

The dissipative coupling in Eq. (S24) indicates that a phase-factor $\theta$ accumulates during photon transport from cavity $b$ to $a$. However, the phase is opposite when the photon traverses in the opposite direction. This exactly maps to the phase acquired by an electron transporting over a path and thus can be usefully interpreted as a Peierls phase, i.e., the line integral of a magnetic gauge potential.

For the two dimensional model shown in Fig. 1 in the main text, the time-reversal operation $\mathcal{T}$ transforms a z-independent operator to its complex conjugate (i.e., exchange $i \leftrightarrow -i$), while the parity operator $\mathcal{P}$ exchanges locations of the modes (exchange $a \leftrightarrow b$). Thus, it is easy to verify that the coherent coupling Hamiltonian in Eq. (S23) is $\mathcal{PT}$-symmetric, i.e.,

$$(\mathcal{PT})\, H_{\text{s}}\, (\mathcal{PT})^{-1} = H_{\text{a}}. \tag{S25}$$

However, for the dissipative coupling Hamiltonian in Eq. (S24), applying $\mathcal{PT}$-transform, we find that the dissipative coupling in Eq. (S23) is anti-$\mathcal{PT}$-symmetric, i.e.,

$$(\mathcal{PT})\, H_{\text{a}}\, (\mathcal{PT})^{-1} = -H_{\text{a}}. \tag{S26}$$

In conclusion, the coherent coupling is $\mathcal{PT}$-symmetric. However, the dissipative coupling with a tunable and conjugate phase factor is anti-$\mathcal{PT}$-symmetric.

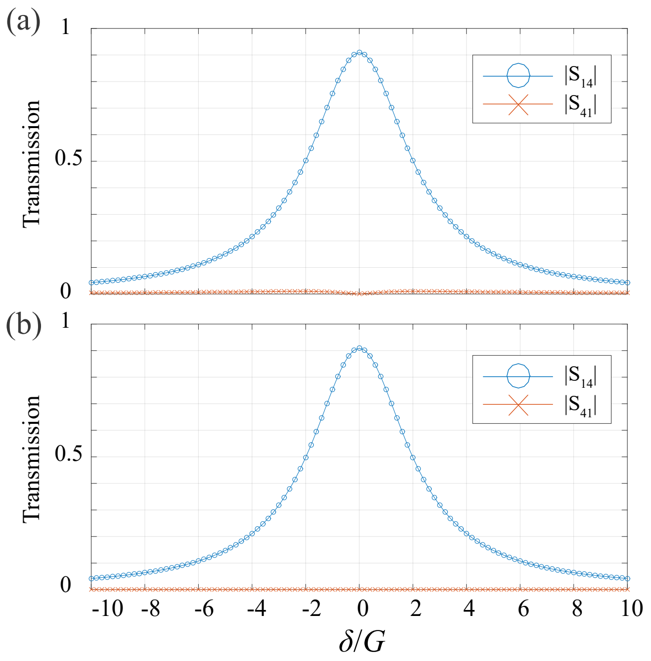


Figure S1: Transmission coefficient between ports 1 and 4 with $\theta = \frac{\pi}{2}$. **a**, calculation using the full Hamiltonian method. **b**, calculation using adiabatically eliminated Hamiltonian.

## 3. The validity of the adiabatic elimination

In the main text, we have discussed the validity of adiabatic elimination in the reversed-dissipation regime by calculating the Riemann sheet structure eigenvalues [Fig. 2 (b) in the main text]. To further verify the validity of the process, in the following, we numerically calculate the unidirectional photon transfer properties with the full Hamiltonian method. Recalling Eq. (2) in the main text, the origin Hamiltonian is

$$\begin{aligned} H &= (\omega - i\kappa)\, a^\dagger a + (\omega - i\kappa)\, b^\dagger b \\ &+ (\omega_m - i\gamma)\, m^\dagger m + G(a^\dagger b + b^\dagger a) \\ &+ G_a(e^{i\theta} a^\dagger m + e^{-i\theta} m^\dagger a) + G_b(b^\dagger m + m^\dagger b). \end{aligned} \tag{S27}$$

The corresponding Langevin equations can be concisely expressed as,

$$\dot{\mu} = -iM\mu + \Gamma\mu_{\rm in}, \tag{S28}$$

where $\mu = [a, b, m]^T$ are the bosonic annihilation operators, $\mu_{\rm in} = [a_{\rm in}, b_{\rm in}, c_{\rm in}]$ are the input noises and $\Gamma = \mathrm{diag}[\sqrt{2\kappa_e}, \sqrt{2\kappa_e}, \sqrt{2\gamma_e}]$ is the external losses matrix. The coefficient matrix is

$$M = \begin{bmatrix} \omega_a - i\kappa & G & G_a e^{i\theta} \\ G & \omega_b - i\kappa & G_b \\ G_a e^{-i\theta} & G_b & \omega_m - i\gamma \end{bmatrix}. \tag{S29}$$

By performing the Fourier transformation, the solution of Eq. (S28) in the frequency domain is,

$$\mu(\omega) = i(M - \omega I)^{-1}\Gamma\mu_{\rm in(\omega)}, \tag{S30}$$

where $I$ denotes the identity matrix. With input-output relation, we can obtain,

$$\begin{aligned} \mu_{\rm out}(\omega) = &\quad \Gamma\mu(\omega) \\ = &\quad \Gamma i(M - \omega I)^{-1}\Gamma\mu_{\rm in}(\omega) \\ = &\quad S(\omega)\mu_{\rm in}(\omega). \end{aligned} \tag{S31}$$

From Eq. S31, it is easy to reach the transmission matrix,

$$S(\omega) = \Gamma i(M - \omega I)^{-1}\Gamma. \tag{S32}$$

For the energy transfer from mode $a$ to $b$ ($b$ to $a$), the transmission coefficient is given by the element $|S_{21}|$ ($|S_{12}|$), which corresponds to the transmission coefficient $|S_{41}|$ ($|S_{41}|$). In Fig. S1 (a), we numerically calculate the transmission using Eq. S32 with $\theta = \frac{\pi}{2}$ and $\gamma = 50\ G$. It is clear that for $\theta = \frac{\pi}{2}$, the energy only transfers from port 4 to 1 but is almost forbidden from 1 to 4. For comparison, we plot the same transmission coefficient using Eq. (12) and Eq. (13) in the main text in Fig. S1 (b) with the same parameters. The two methods show very similar behavior. Hence, our adiabatic elimination is valid for studying the photon transmission in the reversed-dissipation regime.

## References

[1] Y. Y. Gao, B. J. Lester, Y. Zhang, C. Wang, S. Rosenblum, L. Frunzio, L. Jiang, S. Girvin, R. J. Schoelkopf, Programmable interference between two microwave quantum memories, Phys. Rev. X 8 (2) (2018) 021073.

[2] P. Roushan, C. Neill, A. Megrant, Y. Chen, R. Babbush, R. Barends, B. Campbell, Z. Chen, B. Chiaro, A. Dunsworth, et al., Chiral ground-state currents of interacting photons in a synthetic magnetic field, Nat. Phys. 13 (2) (2017) 146–151.
